# Supplementary material for: Coherent coupling of mechanics to a single nuclear spin
Source: arXiv:2107.10961 ancillary file (2021-07-23)
Supplement: Supplementary file 1 [file supplementary.pdf]

# Supplementary information: Coherent coupling of mechanics to a single nuclear spin

Smarak Maity,<sup>1,\*</sup> Benjamin Pingault,<sup>1,2,3,\*</sup> Graham Joe,<sup>1</sup> Michelle Chalupnik,<sup>4</sup>  
Daniel Assumpção,<sup>1</sup> Eliza Cornell,<sup>1</sup> Linbo Shao,<sup>1</sup> and Marko Lončar<sup>1,†</sup>

<sup>1</sup>John A. Paulson School of Engineering and Applied Sciences, Harvard University, Cambridge, MA 02138, USA

<sup>2</sup>QuTech, Delft University of Technology, 2600 GA Delft, The Netherlands

<sup>3</sup>Kavli Institute of Nanoscience Delft, Delft University of Technology, 2600 GA Delft, The Netherlands

<sup>4</sup>Department of Physics, Harvard University, Cambridge, MA 02138, USA

## I. Optical characterization of the SiV

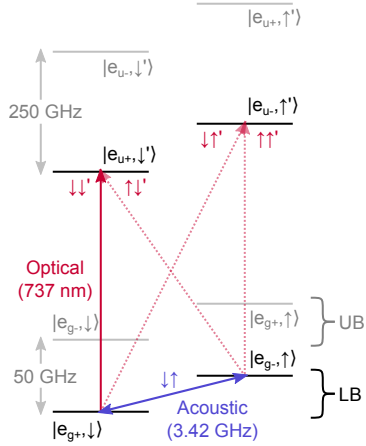

Supplementary Figure 1. Electronic structure of the SiV under an external magnetic field of 0.13 T. The states  $|\downarrow\rangle$  and  $|\uparrow\rangle$  in the main text correspond to  $|e_{g+}, \downarrow\rangle$  and  $|e_{g-}, \uparrow\rangle$  respectively, while  $|\downarrow'\rangle$  and  $|\uparrow'\rangle$  correspond to  $|e_{u+}, \downarrow\rangle$  and  $|e_{u-}, \uparrow\rangle$ . UB and LB indicate the upper and lower branches of the ground-state manifold, respectively.

The complete electronic structure of the SiV under an external magnetic field is shown in Supplementary Fig. 1. A detailed description may be found in [1, 2]. We use a magnetic field with a magnitude of 0.13 T, oriented at an angle of  $90^\circ$  with respect to the axis of the SiV. At temperatures below  $\sim 200$  mK, only the lower branch of the ground-state manifold is populated, allowing the electronic structure to be simplified, as shown in Fig. 1(b) of the main text.

Due to the long spin lifetime at temperatures below  $\sim 200$  mK and the short optical pumping time (100s of ns) under an off-axis magnetic field, continuous resonant excitation of individual optical transitions results in little measurable fluorescence. For example, exciting the  $\downarrow\downarrow'$  transition optically pumps the SiV into  $|\uparrow\rangle$ , limiting the fluorescence at steady state. To observe the optical transitions and deduce the ground-state spin splitting,

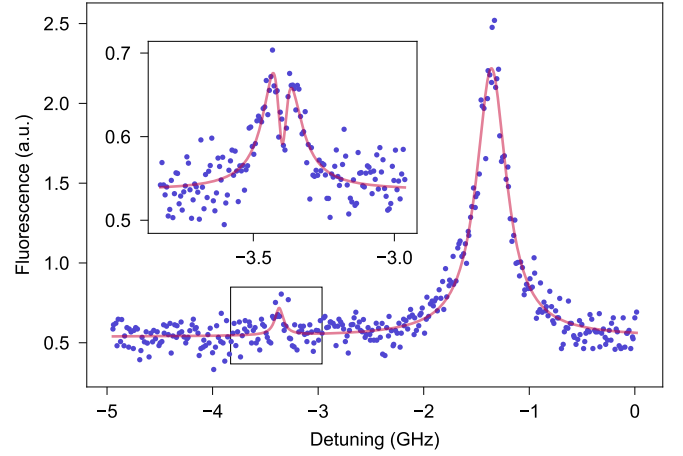

Supplementary Figure 2. Resonant excitation spectrum of the SiV at  $\approx 100$  mK, using two lasers. One laser is resonant with the  $\uparrow\uparrow'$  transition (737.10103 nm), while the second laser is scanned across the  $\downarrow\uparrow'$  and  $\downarrow\downarrow'$  transitions. The horizontal axis represents the detuning of the second laser from the first. Inset: higher-resolution scan of the boxed region, showing a fluorescence dip due to coherent population trapping.

two lasers resonant with two different optical transitions are required. Supplementary Fig. 2 shows a resonant excitation spectrum when one of the lasers is resonant with the  $\uparrow\uparrow'$  transition, while the other laser is scanned across the  $\downarrow\uparrow'$  and  $\downarrow\downarrow'$  transitions. When the second laser is resonant with  $\downarrow\uparrow'$ , coherent population trapping (CPT) of the SiV spin is observed, as shown in the high-resolution scan in the inset. The CPT dip occurs at a detuning between the two lasers that is equal to the frequency of the  $\downarrow\uparrow$  spin transition.

## II. Acoustic control of the SiV spin

The frequency of the  $\downarrow\uparrow$  transition is measured using optically detected acoustic resonance (ODAR). An optical pulse resonant with the  $\uparrow\uparrow'$  transition first resets the system, by pumping the SiV into  $|\downarrow\rangle$  (Supplementary Fig. 3). Then an initialization optical pulse, resonant with  $\downarrow\downarrow'$ , initializes the SiV into  $|\uparrow\rangle$ . An acoustic pulse of duration 20 ns and varying frequency transfers some of the population back into  $|\downarrow\rangle$ , before the population in  $|\downarrow\rangle$  is read out with a second optical pulse resonant with

\* These authors contributed equally.

† loncar@seas.harvard.edu

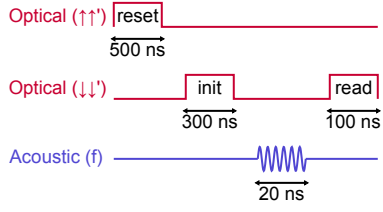

Supplementary Figure 3. Pulse sequence for optically detected acoustic resonance (ODAR).

$\downarrow\downarrow'$ . A histogram of the emitted fluorescence photons is recorded during the entire sequence, as shown in Supplementary Fig. 4.

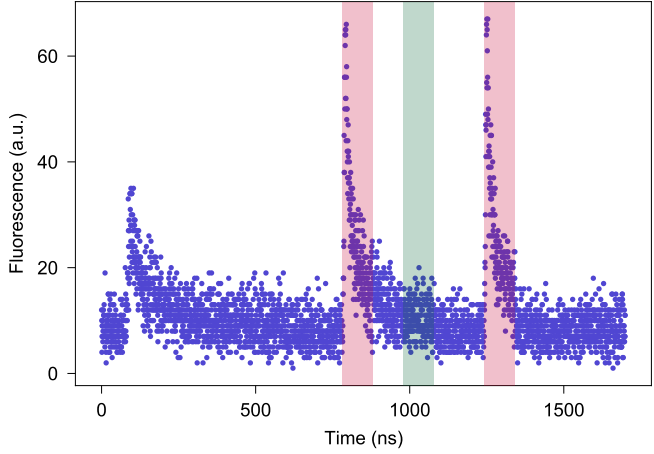

Supplementary Figure 4. Histogram of photon arrival times during the ODAR pulse sequence depicted in Supplementary Fig. 3, accumulated for 60 s. Photon counts are integrated during the first 100 ns of the optical initialization and read-out pulses, indicated by the red shaded regions. Background counts, indicated by the green shaded region, are subtracted from the total counts.

The fluorescence photon counts during the first 100 ns of the initialization and readout pulses are integrated to obtain the initialization and readout counts (red shaded regions in Supplementary Fig. 4). The fluorescence during the last 100 ns of the initialization pulse (green shaded region) is integrated to obtain the background fluorescence counts once the SiV spin has been initialized. The final population in  $|\downarrow\rangle$  after the acoustic pulse is calculated as

$$\text{population in } |\downarrow\rangle = \frac{\text{read. counts} - \text{b.g. counts}}{\text{init. counts} - \text{b.g. counts}} \quad (1)$$

As the frequency of the acoustic pulse is varied, the final population in  $|\downarrow\rangle$  shows a peak (Supplementary Fig. 5). The maximum population is obtained when the acoustic frequency is resonant with the frequency  $f_{\downarrow\uparrow}$  of the  $\downarrow\uparrow$  transition. The measurement is repeated after reducing the amplitude  $a$  (in arbitrary units) of the acoustic pulse, while increasing its duration by a factor  $1/a$ .

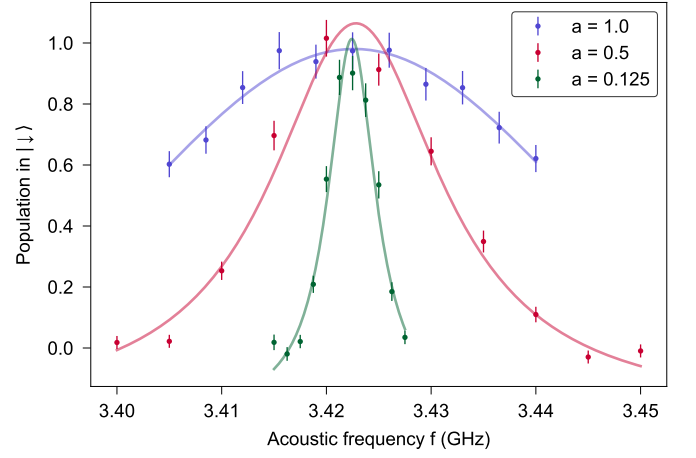

Supplementary Figure 5. Optically detected acoustic resonance of the SiV spin, for different amplitudes  $a$  (in arbitrary units) of the acoustic pulse. The resonance frequency is equal to the frequency of the  $\downarrow\uparrow$  transition.

This makes the pulse spectrally narrower and allows us to determine the spin transition frequency with higher precision. We obtain  $f_{\downarrow\uparrow} = 3.4224 \pm 0.0002$  GHz.

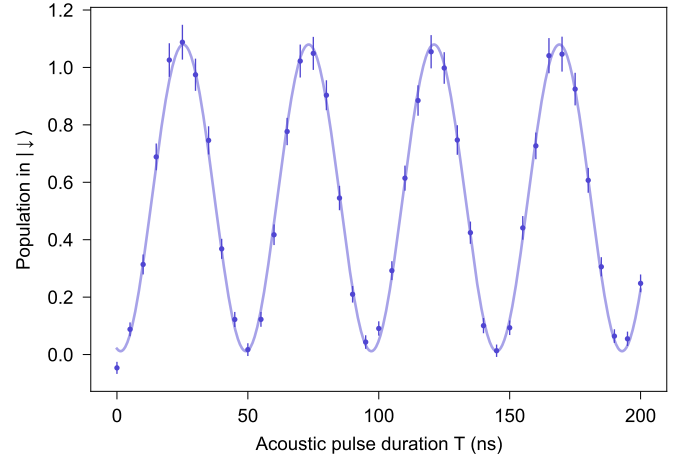

Supplementary Figure 6. Acoustically driven Rabi oscillations of the SiV spin.

With the spin transition frequency identified, we perform acoustically driven Rabi oscillations of the SiV spin. The experimental sequence is the same as that for ODAR, except that the frequency of the acoustic pulse is fixed to  $f_{\downarrow\uparrow}$ , while its duration  $T$  is varied. The observed Rabi oscillations (Supplementary Fig. 6) are fitted with a sinusoid to extract the Rabi frequency  $\Omega = 2\pi \times 20.88$  MHz, resulting in a  $\pi/2$ -pulse duration of  $T_{\pi/2} = 11.97$  ns. Once the Rabi frequency is calibrated, the optical reset pulse is replaced with an acoustic  $\pi$ -pulse for subsequent experiments.

### III. Dynamical decoupling of the SiV spin

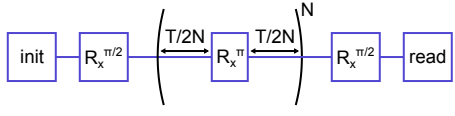

Supplementary Figure 7. CPMG pulse sequence for acoustic dynamical decoupling

We use acoustic Carr-Purcell-Meiboom-Gill (CPMG) pulse sequences (Supplementary Fig. 7) to dynamically decouple the SiV spin from its environment [3]. After optical initialization into  $|\downarrow\rangle$ , an acoustic  $\pi/2$ -pulse puts the SiV spin into a superposition state, which is then subjected to periodically timed  $\pi$ -pulses as it precesses on the equator of the Bloch sphere. A second  $\pi/2$ -pulse projects the SiV spin back onto the  $z$ -axis of the Bloch sphere before the spin population is read out optically.

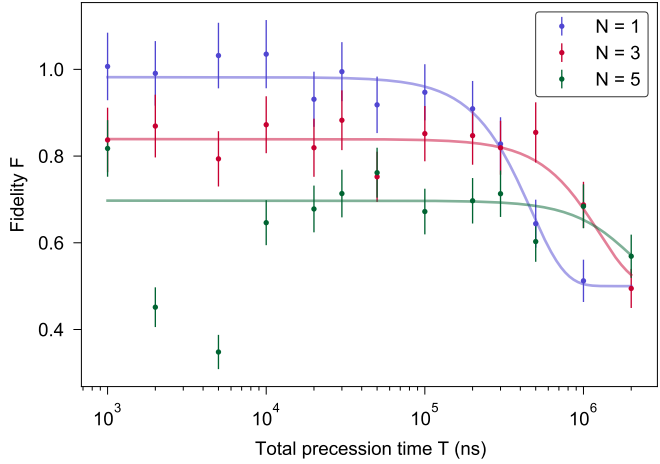

Supplementary Figure 8. Acoustic dynamical decoupling of the SiV spin

The sequence fidelity (measured as the final population in  $|\downarrow\rangle$ ) as a function of the total precession time  $T$  for different numbers of  $\pi$ -pulses  $N$  is shown in Supplementary Fig. 8. Measurements for precession times beyond 2 ms are impractical due to limitations on total experiment time. The observed data are fitted with the model

$$F(T) = \frac{1}{2} + \left(F_0 - \frac{1}{2}\right) e^{-(T/T_2^{\text{CPMG}})^2} \quad (2)$$

to extract the fidelities  $F_0$  at zero delay and the coherence times  $T_2^{\text{CPMG}}$ .

The spin coherence time as a function of the number of CPMG pulses is shown in Supplementary Fig. 9. For  $N = 5$  pulses, we obtain a coherence time  $T_2^{\text{CPMG}} \approx 2$  ms. The base fidelity  $F_0$  decreases with the number of CPMG pulses, due to the accumulation of pulse errors. The XY8 sequences discussed in the main

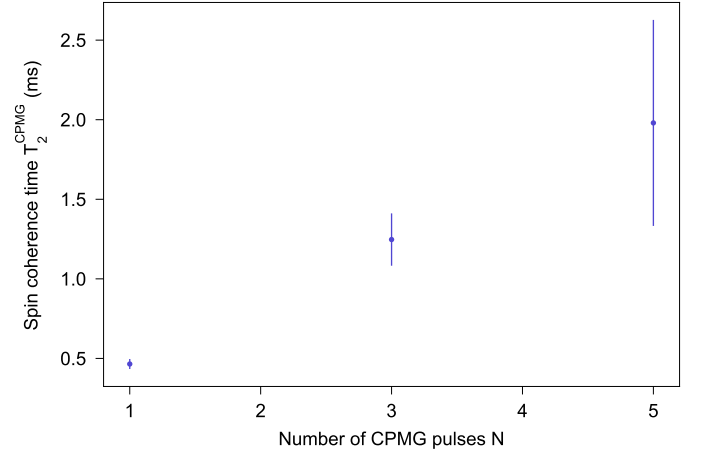

Supplementary Figure 9. SiV spin coherence time v.s. number of CPMG decoupling pulses

text are robust against this type of errors, allowing us to perform XY8 sequences with 16 pulses with no reduction in fidelity. For  $N = 5$  pulses, we observe that the fidelity  $F$  goes below 1/2 for certain values of the total precession time, indicating coherent interaction with nuclear spins in the local environment. This coherent interaction is characterized with higher precision using XY8 sequences as described in the main text.

### IV. Simulation of the electron-nuclear spin system

The Hamiltonian for the SiV electron spin and a single  $^{13}\text{C}$  nuclear spin is

$$\mathcal{H}_0 = 2\pi\hbar S_z^{\text{SiV}} (A_{\parallel} S_z^{\text{nuc}} + A_{\perp} S_x^{\text{nuc}}) + 2\pi\hbar f_L S_z^{\text{nuc}}, \quad (3)$$

in which  $f_L$  is the nuclear Larmor frequency [4]. When no acoustic or optical pulses are applied, the density matrix  $\rho$  of the system undergoes free evolution under  $\mathcal{H}_0$ . The acoustic pulses resonant with  $f_{\downarrow\uparrow}$  rotate the SiV spin around the  $X$  or  $Y$ -axes of the Bloch sphere depending on their phase. Since the rotation angle is  $\pi/2$  over a duration  $T_{\pi/2}$ , the interaction of the acoustic pulses with the SiV spin can therefore be described by the Hamiltonians

$$\mathcal{H}_X = \hbar S_x^{\text{SiV}} \frac{\pi}{2T_{\pi/2}}, \quad (4)$$

$$\mathcal{H}_Y = \hbar S_y^{\text{SiV}} \frac{\pi}{2T_{\pi/2}}. \quad (5)$$

For the duration of the acoustic pulse, the system evolves under  $\mathcal{H}_0 + \mathcal{H}_X$  or  $\mathcal{H}_0 + \mathcal{H}_Y$ .

An optical pulse resonant with  $\downarrow\downarrow'$  optically pumps the SiV into  $|\uparrow\rangle$ . The effect on the density matrix  $\rho$  is given by the operation

$$|\uparrow\rangle_{\text{SiV}} \langle\uparrow|_{\text{SiV}} \otimes \text{Tr}_{\text{SiV}}(\rho) \quad (6)$$

in which  $\text{Tr}_{\text{SiV}}$  represents a partial trace over the SiV spin degrees of freedom. The experimental sequences in the main text are simulated numerically using the Hamiltonians and operations described above, with the nuclear spin starting in a mixed state.

### V. Expression for nuclear spin resonances

Nuclear spin resonances occur when the value of the inter-pulse time  $\tau$  in the XY8 sequence is such that the nuclear spin undergoes a conditional rotation, leading to a collapse in fidelity. From Fig. 1d of the main text, we expect conditional rotations to occur when the nuclear spin undergoes precession by an angle  $\pi$  before an SiV spin flip, causing it to increase its polar angle on the Bloch sphere. The nuclear precession frequencies when the SiV is in  $|\uparrow\rangle$  or  $|\downarrow\rangle$  are

$$f_{\uparrow} = \sqrt{\left(f_L + \frac{A_{\parallel}}{2}\right)^2 + \frac{A_{\perp}^2}{4}}, \quad (7)$$

$$f_{\downarrow} = \sqrt{\left(f_L - \frac{A_{\parallel}}{2}\right)^2 + \frac{A_{\perp}^2}{4}}. \quad (8)$$

Assuming  $A_{\parallel}, A_{\perp} \ll f_L$ , using the Taylor expansion  $\sqrt{1+x} \approx 1+x/2-x^2/8$ , and keeping terms up to second order, these can be simplified to obtain

$$f_{\uparrow} = f_L \sqrt{\left(1 + \frac{A_{\parallel}}{2f_L}\right)^2 + \frac{A_{\perp}^2}{4f_L^2}} \quad (9)$$

$$= f_L \sqrt{1 + \frac{A_{\parallel}}{f_L} + \frac{A_{\parallel}^2 + A_{\perp}^2}{4f_L^2}} \quad (10)$$

$$\approx f_L \left[ 1 + \frac{1}{2} \left( \frac{A_{\parallel}}{f_L} + \frac{A_{\parallel}^2 + A_{\perp}^2}{4f_L^2} \right) - \frac{1}{8} \left( \frac{A_{\parallel}}{f_L} \right)^2 \right] \quad (11)$$

$$= f_L \left[ 1 + \frac{A_{\parallel}}{2f_L} + \frac{A_{\perp}^2}{8f_L^2} \right], \quad (12)$$

and

$$f_{\downarrow} \approx f_L \left[ 1 - \frac{A_{\parallel}}{2f_L} + \frac{A_{\perp}^2}{8f_L^2} \right]. \quad (13)$$

The average nuclear precession frequency is

$$f_{\text{avg}} = \frac{f_{\uparrow} + f_{\downarrow}}{2} \approx f_L \left[ 1 + \frac{A_{\perp}^2}{8f_L^2} \right]. \quad (14)$$

The time between two spin flips is  $2\tau$ , so the resonance condition is

$$2\pi f_{\text{avg}} \times 2\tau \approx (2k+1)\pi \quad (15)$$

$$4\pi f_L \left[ 1 + \frac{A_{\perp}^2}{8f_L^2} \right] \tau \approx (2k+1)\pi \quad (16)$$

$$\tau \approx \frac{2k+1}{4f_L} \left[ 1 - \frac{A_{\perp}^2}{8f_L^2} \right]. \quad (17)$$

### VI. Modelling of the nuclear spin system

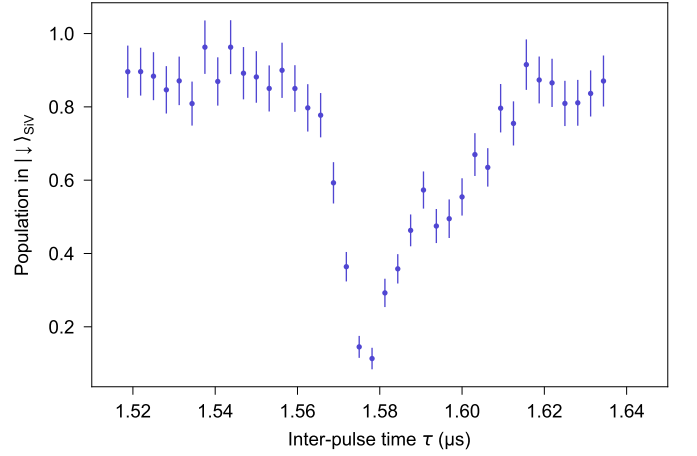

Supplementary Figure 10. Close-up of the experimentally measured nuclear spin resonance dip around  $\tau = 1.578 \mu\text{s}$ .

The nuclear spin resonance dips are slightly asymmetric (Supplementary Fig. 10), suggesting that there are additional nuclear spins with resonance times close to that of the target nuclear spin. We approximate the effect of these spins with a single additional nuclear spin in our model. The parameters of the model are optimized by minimizing the mean squared error between the model and the experimental data for nuclear spin resonance, nuclear spin initialization, and the nuclear Ramsey precession frequencies. We obtain the parameters

$$\{A_{\parallel}, A_{\perp}\}_{\text{target}} = \{0.1143 \text{ MHz}, 0.3277 \text{ MHz}\} \quad (18)$$

$$\{A_{\parallel}, A_{\perp}\}_{\text{parasitic}} = \{0.0840 \text{ MHz}, 0.1370 \text{ MHz}\} \quad (19)$$

for the two nuclear spins in our model.

The second nuclear spin impacts the fidelity of initialization and readout for the target nuclear spin. The initialization fidelity is defined as  $F_{\text{init}} = |\langle \psi_{\text{nuc}}^{\text{target}} | \psi_{\text{nuc}} \rangle|^2$ , in which  $|\psi_{\text{nuc}}^{\text{target}}\rangle$  is the desired nuclear spin state, and  $|\psi_{\text{nuc}}\rangle$  is the state of the nuclear spin at the end of the initialization sequence. Since the readout sequence contains the same operations as the initialization sequence but in reverse, the readout fidelity is equal to the initialization fidelity, hence the total sequence fidelity is  $F = F_{\text{init}}^2$ . The experimental fidelity for the entire sequence is measured as the population in the final state of the SiV (for  $\tau = 1.569 \mu\text{s}$ ,  $|\uparrow\rangle_{\text{SiV}}$  or  $|\downarrow\rangle_{\text{SiV}}$  for initialization into  $|\uparrow\rangle_{\text{nuc}}$  or  $|\downarrow\rangle_{\text{nuc}}$  respectively). The experimental fidelities for initialization and readout are calculated as the square root of the total fidelity. For a single nuclear spin, the total sequence fidelity is maximized at an inter-pulse time of  $\tau = 1.586 \mu\text{s}$  (Supplementary Fig. 11). However, the presence of the additional spin with a resonance close to this value decreases the fidelity, resulting in the optimum value of  $\tau$  to be  $1.569 \mu\text{s}$ . This agrees with experimental

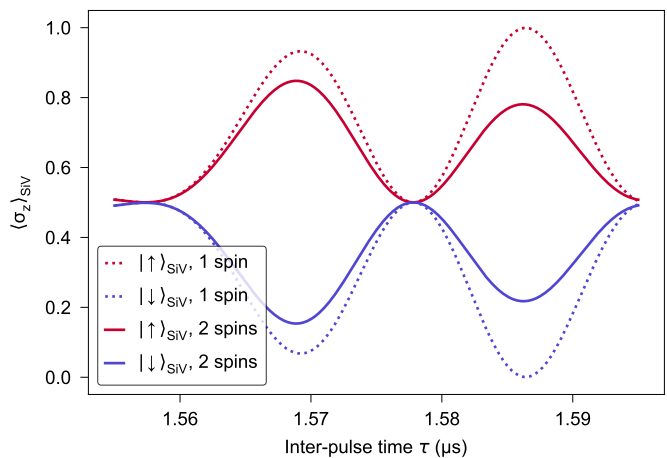

observations (Fig. 3c in the main text).

Supplementary Figure 11. Final SiV spin projection for the nuclear spin initialization and readout sequence as a function of inter-pulse time  $\tau$ , for models with one and two nuclear spins. The presence of the additional nuclear spin reduces the fidelity of the sequence. The curves are labelled by the initial state of the SiV spin, which determines the spin state in which the nuclear spin is initialized, as described in the main text.

- 
- [1] C. Hepp, T. Müller, V. Waselowski, J. N. Becker, B. Pingault, H. Sternschulte, D. Steinmüller-Nethl, A. Gali, J. R. Maze, M. Atatüre, and C. Becher, Electronic structure of the silicon vacancy color center in diamond, *Phys. Rev. Lett.* **112**, 036405 (2014).
  - [2] C. Hepp, *Electronic structure of the silicon vacancy color center in diamond* (2014).
  - [3] M. A. Ali Ahmed, G. A. Álvarez, and D. Suter, Robustness of dynamical decoupling sequences, *Phys. Rev. A* **87**, 042309 (2013).
  - [4] T. H. Taminiau, J. Cramer, T. van der Sar, V. V. Dobrovitski, and R. Hanson, Universal control and error correction in multi-qubit spin registers in diamond, *Nature Nanotechnology* **9**, 171 (2014).
